# Supplementary material for: Combining Neuro-Evolution of Augmenting Topologies with Convolutional Neural Networks
Source: arXiv:2211.16978 source file (2022-10-20)
Supplement: Supplementary file 1 [file studienprotokoll.tex]

\documentclass[11pt]{article}
\setlength{\parindent}{0pt}
\usepackage[utf8]{inputenc}

\title{Studienprotokoll}
\author{Jan Hohenheim, Mathias Fischler, Sara Zarubica, Jeremy Stucki}

\begin{document}

\maketitle
\newpage

\tableofcontents
\newpage

\section{Verantwortlichkeiten}
\subsection{Projektteilnehmer}
Jan Hohenheim \\
Grosswiesenstrasse 153 \\
8051 Zürich \\
079 963 17 64 \\
jan@hohenheim.ch\\

Jeremy Stucki \\
Oberdorf 12 \\
5079 Zeihen \\
076 520 0698 \\
Jeremy.Stucki@stud.bbbaden.ch\\

Mathias Fischler \\
Gänsacker 8 \\
5070 Frick \\
Mathias.Fischler@stud.bbbaden.ch\\

Sara Zarubica \\
Zelgmattstrasse 14 \\
8956 Killwangen \\
076 464 1306 \\
Sara.Zarubica@stud.bbbaden.ch\\

\subsection{Beteiligte Institution}
Berufsfachschule BBB \\
Wiesenstrasse 32 \\
5400 Baden \\
056 222 0206 \\
sekretariat@bbbaden.ch\\
\newpage

\section{Das Projekt}
\subsection{Definition des Projektes}
In unserem Projekt wollen wir anhand von künstlicher Intelligenz Mammographien beurteilen können.

Dazu verwenden wir die de dato nicht kombinierten Technologien NeuroEvolution of Augmenting Topologies (NEAT) und Convolutional Neural Networks (CNN).

Der Benutzer ladet eine Mammografie hoch, die er in digitaler Form (z.B. als
.png oder .bmp) auf seinem Rechner zur Verfügung hat. Die Software gibt
darauf hin aus, wie wahrscheinlich die geprüfte Brust von Krebs befallen ist.

Unsere Software kann Ärzte bei Zweifelsfällen einer Diagnose unterstützen,
kann diese aber keinesfalls ersetzen.

Privatpersonen können die Software für
präventive Selbstuntersuchungen nutzen.
Unsere Zielgruppe sind Ärzte, Radiologen und zum Teil Privatpersonen.

\subsection{Hintergrund des Projektes}
Im Rahmen unserer Projektarbeit haben wir uns für diese Arbeit entschieden, da uns dieses Themengebiet interessiert und wir Potenzial bei der Kombination von verschiedenen vorhandenen Technologien sehen.

\subsection{Nutzen und Risiko}
Unsere Software kann Ärzte bei Zweifelsfällen einer Diagnose unterstützen,
kann diese aber keinesfalls ersetzen.

Privatpersonen, die über Mammografien verfügen, können die Software für
präventive Selbstuntersuchungen nutzen und je nach Ergebnis einen Arzt
kontaktieren.

Zu dem Risiko gehört vor allem die Aussagekraft des Resultats. Damit ist gemeint, dass das Resultat nicht 100 Prozentig ausschlaggebend ist und den Arzt nicht ersetzen kann.
\newpage
\subsection{Unsere Ziele}
Zu unseren Zielen gehören:

\begin{itemize}
	\item{Das Einlesen von Mammographien}
	\item{Die Beurteilung von Mammographien}
	\item{Die Visuelle Darstellung von den generierten neuronalen Netzwerken}
	\item{Die Platzformunabhängigkeit}
\end{itemize}
\subsection{Projektdauer}
Vom 17.09.2016 bis zum 18.01.2017

\end{document}
